# Supplementary material for: Synthesis of passive lossless metasurfaces using auxiliary fields for reflectionless beam splitting and perfect reflection
Source: arXiv:1607.02954 ancillary file (2016-07-19)
Supplement: Supplementary file 1 [file Supplemental_Material_Final.pdf]

# SUPPLEMENTAL MATERIAL

*"SYNTHESIS OF PASSIVE LOSSLESS METASURFACES WITH AUXILIARY FIELDS FOR REFLECTIONLESS WIDE-ANGLE BEAM SPLITTING AND PERFECT REFLECTION"*, BY ARIEL EPSTEIN AND GEORGE V. ELEFTHERIADES

## 1 SELF-CONSISTENT EVOLUTION OF AUXILIARY FIELDS

The metasurfaces designed in the main text have been verified via full-wave simulations using periodic boundary conditions. To verify that no external power sources are required to generate the auxiliary fields, and that they are induced self-consistently by the passive lossless metasurface, we simulated finite metasurface structures and excited them using a finite-width Gaussian beam.

### 1.1 REFLECTIONLESS WIDE-ANGLE BEAM SPLITTER

For the first application of reflectionless beam splitting, we have implemented a metasurface consisting of 12 replicas of the single-period structure presented in Fig. 1 of the main text (total length of $L=(1200/95)\lambda$). The metasurface was placed symmetrically with respect to the origin, and a Gaussian beam with electric field amplitude $E_{\mathrm{in}}$ and beam waist of $6\lambda$, centered at $(y,z)=(0,0)$, was launched at the metasurface from below. The simulation domain was $(y,z)\in[-8.5\lambda,8.5\lambda]\times[-2\lambda,4\lambda]$ to allow proper visualization of the evolution of the scattered fields.

The simulated field distribution $\left|\Re\left\{E_x(y,z)\right\}\right|$ is presented in Fig. S1(a). The evolution of the auxiliary surface waves due to the interaction between the Gaussian beam and the metasurface elements is clearly observed below the metasurface. Above the metasurface, the expected interference pattern between the two beams propagating towards $\pm 71.81°$ indeed appears. Outside the metasurface aperture, towards the top right and left corners of the simulation domain, the formation of two distinctive phase fronts can be seen, slightly distorted due to the interference with the tail of the exciting Gaussian beam.

To get a clearer comparison to the results presented in Fig. 1 of the main text, we show in Fig. S1(b) a close-up of the simulation domain around the center of the Gaussian beam [white frame in Fig. S1(a)]. In this region the excitation best

resembles a plane wave (phase fronts are parallel to the surface), and the edge effects (not taken into account in the theoretical derivation presented in the paper) should be minor. Indeed, when comparing Fig. S1(b) with Fig. 1(b) and (c) of the main text, very good agreement is observed (note that the color axis in both figures is identical).

Similar agreement is achieved for the z-directed real power $P_z(y,z)$ presented in Fig. S1(c). The close-up in Fig. S1(d) also compares very well with Fig. 1(d) and (e) of the main text. The differences at the top of the plot, close to $z=\lambda$, are due to the fact that the two beams above the metasurface are not plane waves now, but also feature a finite beam width (corresponding to the excitation). Thus, they cannot form the interference pattern indefinitely as in the theoretical derivation, but also in the region where they overlap.

To further highlight the evolution of the scattered fields, we illustrate in Fig. S1(e) the propagation of the various modes [superimposed on the fields distribution of Fig. S1(a)]; this is slightly hard to observe in Fig. S1(a) due to interference effects. White-filled arrows correspond to the incident beam, the right and left propagating beams have light-red and light-green fillings, respectively, and the auxiliary surface waves are represented by orange-filled arrows. The arrow widths qualitatively correspond to the field amplitude of the respective modes, spatially varying due to the finite nature of the excitation. This clarifies how the diffracted modes supported by the finite aperture, and elucidates the variations in field magnitude.

Importantly, it is obvious from these results that the auxiliary fields are self-generated by the reactive metasurface, and no external excitation (other than the incident beam) is required for achieving the desirable functionality. In addition, integrating over the power radiated to the far field, each of the diffracted beams, it is confirmed that 48.5% of the incident power is successfully coupled to each beam, 1% is specularly reflected, and another 2% are scattered otherwise. The slightly-reduced performance with respect to a plane-wave excitation is expected, as Gaussian beams do not form perfectly-planar phase fronts.

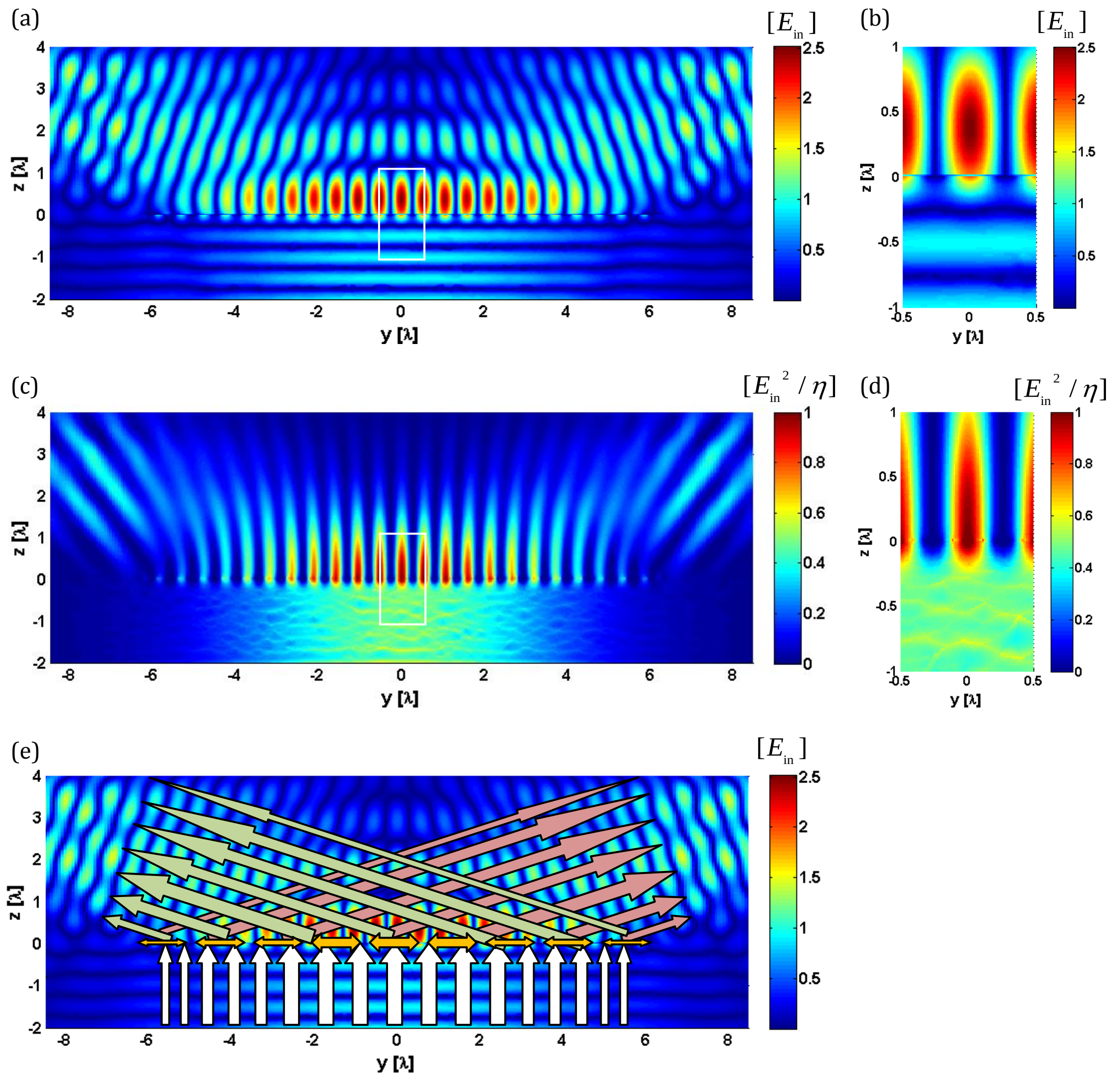


**Figure S1.** Simulated results for a finite (12-period long) beam-splitting metasurface excited by a normally-incident Gaussian beam centered at $(y,z)=(0,0)$ having a beam waist of $6\lambda$. (a) Simulated field distribution $\left|\Re\left\{E_x(y,z)\right\}\right|$. (b) Close-up on the white-framed region in (a). (c) Simulated z-directed real Poynting vector $P_z(y,z)$. (d) Close-up on the white-framed region in (c). (e) Propagation of the various modes. White-filled arrows correspond to incident fields, light red and light green filling to right and left propagating splitted beams, respectively, and the auxiliary surface waves are represented by orange-filled arrows. Arrow widths qualitatively correspond to field amplitude in the different regions.

## 1.2 PERFECT ENGINEERED REFLECTION

For the second application considered in the paper, perflect engineered reflection, we have again implemented a metasurface consisting of 20 replicas of the single-period structure presented in Fig. 2 of the main text (total length of $L=(2000/95)\lambda$). The metasurface was placed symmetrically with respect to the origin, and a Gaussian beam with electric field amplitude $E_{\mathrm{in}}$ and beam waist of $10\lambda$, centered at $(y,z)=(0,0)$, was launched at the metasurface from below. The simulation domain was $(y,z)\in[-12.5\lambda,12.5\lambda]\times[-10\lambda,2\lambda]$ to allow proper visualization of the evolution of the scattered fields.

As in this application power is asymmetrically diverted from the normally incident beam to establish the beam departing at $\theta_{\mathrm{out}}=71.81°$, edge effects originating from the finite excitation beam waist and finite metasurface size have a larger effect than for the beam-splitting metasurface. To allow the evolution of the reflected beam, power is carried over the metasurface from left (negative $y$ region) to right (positive $y$ region) while radiating, in some similarity to leaky wave antennas (this property was termed "non locality" in Ref. 24). Thus, we chose to simulate a larger metasurface and extend the Gaussian beam waist to allow a sufficient area for build-up of the diffracted mode.

The simulated field distribution $\left|\Re\left\{E_x\left(y,z\right)\right\}\right|$ is presented in Fig. S2(a). As can be seen therein, the interaction between the Gaussian beam and the metasurface gives rise to the auxiliary surface waves, propagating on the top facet of the metasurface from left to right. This interaction contributes to the build-up of the reflected beam, growing stronger and stronger as one approaches the center of the incident Gaussian beam. As for the case of the beam-splitting metasurface, we zoom in on a single period in the vicinity of the origin [white frame in Fig. S2(a)], and present the corresponding field distribution in Fig. S2(b). In that region edge effects are minor, and the field distribution is in excellent agreement with the one simulated for an infinite metasurface excited by a normally-incident plane wave [Fig. 2(c) of the main text].

Similar conclusions can be drawn from the z-directed real Poynting vector plots, presented in Fig. S2(c) and (d). Once again, the close-up on the white-framed region in Fig. S2(c) which is presented in Fig. S2(d) agrees very well with the simulated results for the infinite structure [Fig. 2(e) of the main text].

As for the beam-splitting metasurface, it is hard to visualize the power flow due to the interference between the incident and scattered fields. Therefore, we present in Fig. S2(e) an illustration that elucidates the evolution of the diffracted modes [superimposed on the field distribution of Fig. S2(a)]. White-filled arrows represent the incident Guassian beam, while light-red filling corresponds to the reflected beam, and orange-filled arrows to the auxiliary surface waves; the arrow widths qualitatively correspond to the spatially-varying field amplitudes. This plot further clarifies the need in a larger metasurface and beam waist to achieve proper generation of the reflected beam. As the power impinging the leftmost edge of the metasurface arrives from the tail of the incident Gaussian beam, the auxiliary surface waves evolving there have a relatively small amplitude. The field induced on the bottom facet to promote the evolution of the reflected beam are thus small in this area. As the excitation fields grow towards the center of the normally-incident Gaussian beam, the power carried from left to right by the surface waves collectively contributes to the increase in amplitude of the reflected beam. Towards the rightmost part of the metasurface (the other tail of the Gaussian beam), the amplitude decreases again, in correspondence with the finite width of the reflected beam.

Once more, these results unambiguously demonstrate that the auxiliary fields are self-generated by the reactive metasurface, and no external excitation (other than the incident beam) is required for achieving the desirable functionality. The angular distribution of the power in the far field confirms that 95% of the scattered power is coupled to the reflected beam propagating towards $\theta = 71.81°$, 1.5% is coupled to the conjugate mode propagating towards $\theta = -71.81°$, 1.5% is specularly reflected, and another 2% are scattered otherwise. Noticeably, no fields are radiated to the region above the metasurface. The reduction in performance with respect to a plane-wave excitation is slightly larger here than for the beam splitter, as the "non local" nature of the metasurface makes it more prone to edge effects due the finite extent of the Gaussian beam. Nevertheless, it was observed that as the incident beam waist and metasurface length increase, the coupling efficiency to the desirable mode improves, as expected.

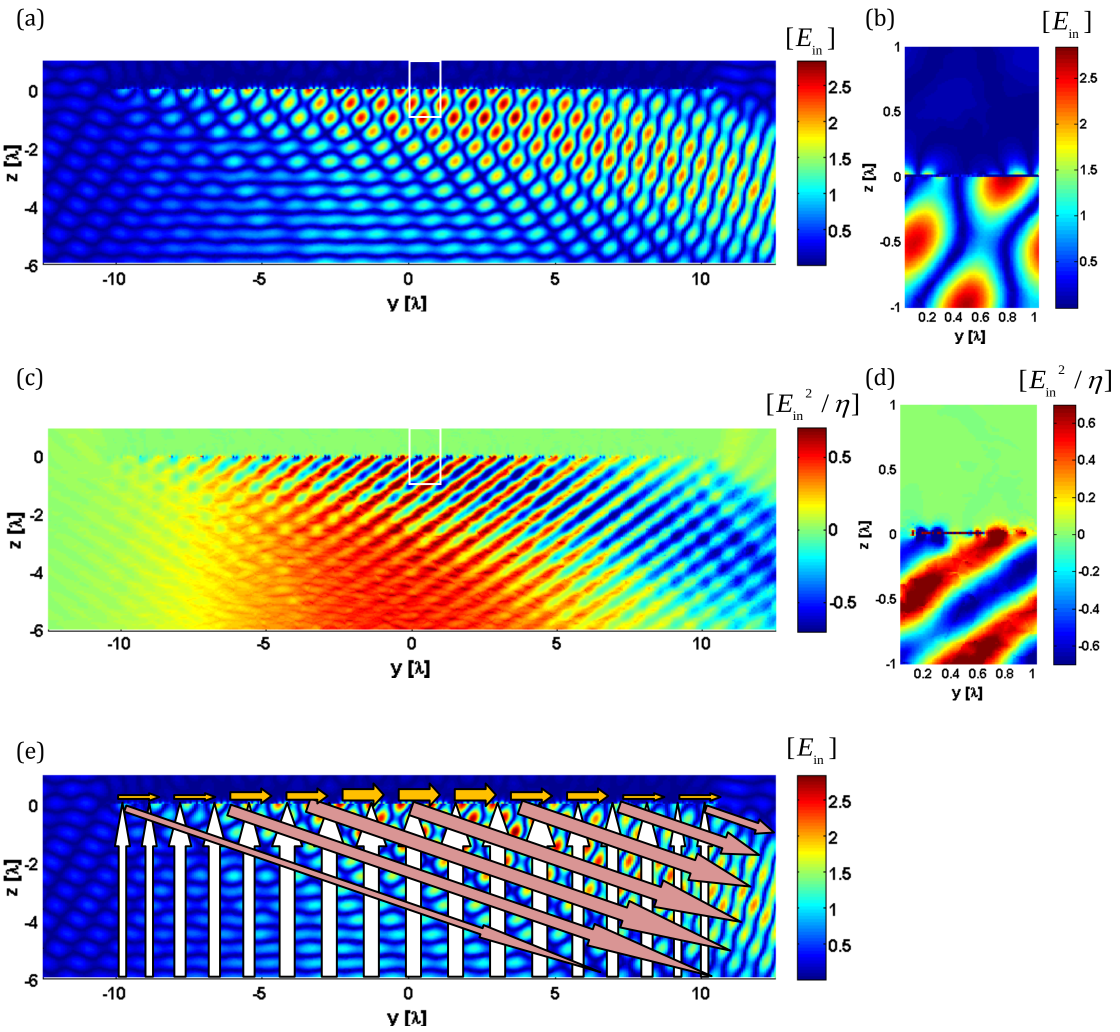


**Figure S2.** Simulated results for a finite (20-period long) perfect reflection metasurface excited by a normally-incident Gaussian beam centered at $(y,z)=(0,0)$ having a beam waist of $10\lambda$. (a) Simulated field distribution $\left|\Re\left\{E_x\left(y,z\right)\right\}\right|$. (b) Close-up on the white-framed region in (a). (c) Simulated z-directed real Poynting vector $P_z\left(y,z\right)$. (d) Close-up on the white-framed region in (c). (e) Propagation of the various modes. White-filled arrows correspond to incident fields, light red filling to the reflected beam, and the auxiliary surface waves are represented by orange-filled arrows. Arrow widths qualitatively correspond to field amplitude in the different regions.

# 2 METASURFACE IMPLEMENTATION IN ANSYS HFSS

To implement the specified metasurfaces in ANSYS HFSS, we utilize the scheme developed in Refs. 20, 21 of the paper, using three cascaded reactance sheets supported by a two laminates of thickness $t$, permittivity $\varepsilon_{\text{sub}}$, and permeability $\mu_{\text{sub}}$ [Fig. S3(a)].

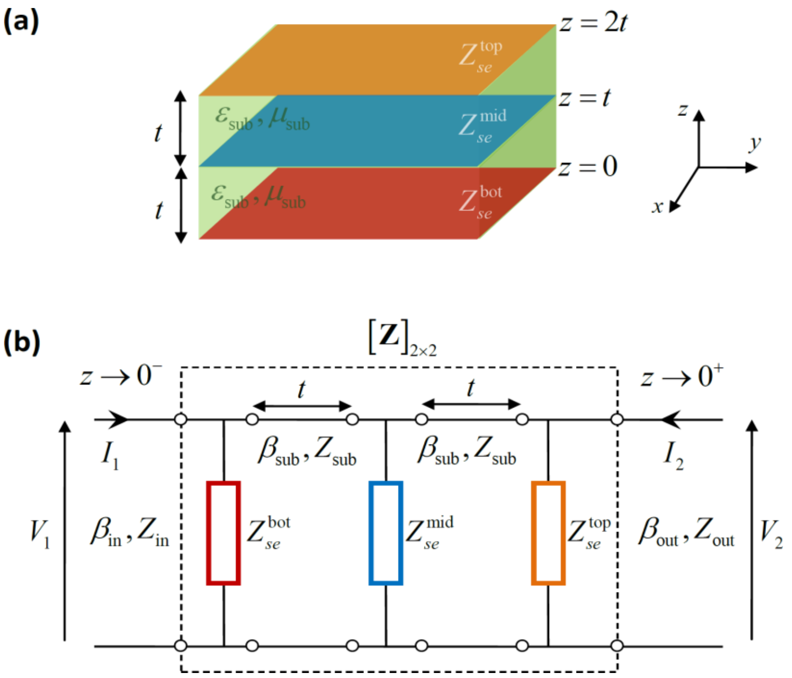


**Figure S3.** (a) Three-layer impedance sheet structure implementing a general omega-type bianisotropic meta-atom. (b) The corresponding equivalent transmission line model.

Considering an infinite periodic array of this unit cell, one can use a transmission line model [Fig. S3(b)] to evaluate the equivalent impedance matrix

(S1) $$[\mathbf{Z}] = \begin{pmatrix} Z_{11} & Z_{12} \\ Z_{21} & Z_{22} \end{pmatrix}$$

for the surface, assuming a normally-incident plane wave is impinging the structure from below. For the evaluation, the longitudinal wavenumber $\beta_{\text{sub}}$ and wave impedance $Z_{\text{sub}}$ in the laminates are given by

(S2) $$\beta_{\text{sub}} = \omega\sqrt{\mu_{\text{sub}}\varepsilon_{\text{sub}}}, \quad Z_{\text{sub}} = \sqrt{\mu_{\text{sub}} / \varepsilon_{\text{sub}}}$$

The relations between the tangential fields implied by the matrix of Eq. (S1) are given, by definition, via

(S3)
$$\begin{pmatrix} E_x^- \\ E_x^+ \end{pmatrix} = \begin{pmatrix} Z_{11} & Z_{12} \\ Z_{21} & Z_{22} \end{pmatrix} \begin{pmatrix} H_y^- \\ -H_y^+ \end{pmatrix},$$

where $E_x^{\pm}(y), H_y^{\pm}(y)$ are as defined in the main text. These, in turn, can be compared to the omega-biaisotropic sheet transition conditions [Eq. (1) of the main text], yielding the following relation between the matrix elements and the metasurface constituents,

(S4)
$$\begin{cases} Z_{11} = Z_{se} + \dfrac{(1+2K_{em})^2}{4Y_{sm}} \\ Z_{12} = Z_{21} = Z_{se} - \dfrac{(1-2K_{em})(1+2K_{em})}{4Y_{sm}} \\ Z_{22} = Z_{se} + \dfrac{(1-2K_{em})^2}{4Y_{sm}} \end{cases}.$$

Note that if the metasurface constituents represent a passive and lossless design $\Re\{Z_{\mathrm{se}}\} = \Re\{Y_{\mathrm{sm}}\} = \Im\{K_{\mathrm{em}}\} = 0$, then the matrix elements are purely imaginary. Using the transmission line model of Fig. S3(b), the sheet impedances that would implement a given impedance matrix as in Eq. (S4) can be assessed analytically, yielding

(S5)
$$\begin{cases} Z_{\mathrm{se}}^{\mathrm{bot}} = \dfrac{Z_{\mathrm{sub}} \tan(\beta_{\mathrm{sub}} t)}{j + Z_{\mathrm{sub}} \tan(\beta_{\mathrm{sub}} t) \dfrac{Z_{22}+Z_{12}}{\Delta_Z}} \\ Z_{\mathrm{se}}^{\mathrm{mid}} = \dfrac{\left[Z_{\mathrm{sub}} \tan(\beta_{\mathrm{sub}} t)\right]^2 \dfrac{Z_{12}}{\Delta_Z}}{2jZ_{\mathrm{sub}} \tan(\beta_{\mathrm{sub}} t) \dfrac{Z_{12}}{\Delta_Z} - \sec^2(\beta_{\mathrm{sub}} t)} \\ Z_{\mathrm{se}}^{\mathrm{top}} = \dfrac{Z_{\mathrm{sub}} \tan(\beta_{\mathrm{sub}} t)}{j + Z_{\mathrm{sub}} \tan(\beta_{\mathrm{sub}} t) \dfrac{Z_{11}+Z_{12}}{\Delta_Z}} \end{cases},$$

where $\Delta_Z = Z_{11}Z_{22} - Z_{12}Z_{21}$ is the determinant of the matrix $[\mathbf{Z}]$. Once more, for a passive and lossless design $Z_{ij}$ are purely imaginary, which leads [via Eq. (S5)] to reactive $Z_{\mathrm{se}}^{\mathrm{bot}}, Z_{\mathrm{se}}^{\mathrm{mid}}, Z_{\mathrm{se}}^{\mathrm{top}}$, as required.

In view of the derivation in Eqs. (S1)-(S5), the passive lossless metasurface elements can be implemented in ANSYS HFSS as unit cells consisting of three reactive sheets. The continuous design specifications $Z_{se}(y), Y_{sm}(y), K_{em}(y)$ are discretized in intervals of $\Delta y$. At each point $y_n = n\Delta y, n \in \mathbb{Z}$ on the metasurface aperture, the local specifications of $Z_{se}(y_n), Y_{sm}(y_n), K_{em}(y_n)$ are used to evaluate $[\mathbf{Z}]$ via Eq. (S4), and subsequently the required reactance values of the unit cell at $y$ via Eq. (S5). The typical local periodicity assumption is used, and the process is repeated for each unit cell to form the complete metasurface. Impedance Boundary Conditions feature is used in ANSYS HFSS to implement the individual reactive sheets for simulation purposes.

For the metasurfaces presented in the paper, the Rogers RO3010 was chosen as the laminate in Fig. S3, featuring permittivity of $\varepsilon_{\mathrm{sub}} = 13.06\varepsilon_0$ and permeability $\mu_{\mathrm{sub}} = \mu_0$ at the design frequency $f = 20\mathrm{GHz}$ ($\varepsilon_0$ and $\mu_0$ are the permittivity and permeability of vacuum, respectively). The laminate thickness was $t = 5\mathrm{mil} \approx \lambda/118$, and the unit cell size was $\Delta y = \lambda/9.5 \approx 1.58\mathrm{mm}$.

For reference, Fig. S4 presents the metasurface constituents [Fig. S4(a) and (b)] and corresponding reactance values $X_{\mathrm{se}} = \Im\{Z_{\mathrm{se}}\}$ [Fig. S4(c) and (d)] associated with the beam splitter [Fig. S4(a) and (c)] and perfect reflection [Fig. S4(b) and (d)] applications. As the metasurfaces are periodic, only one period is presented.

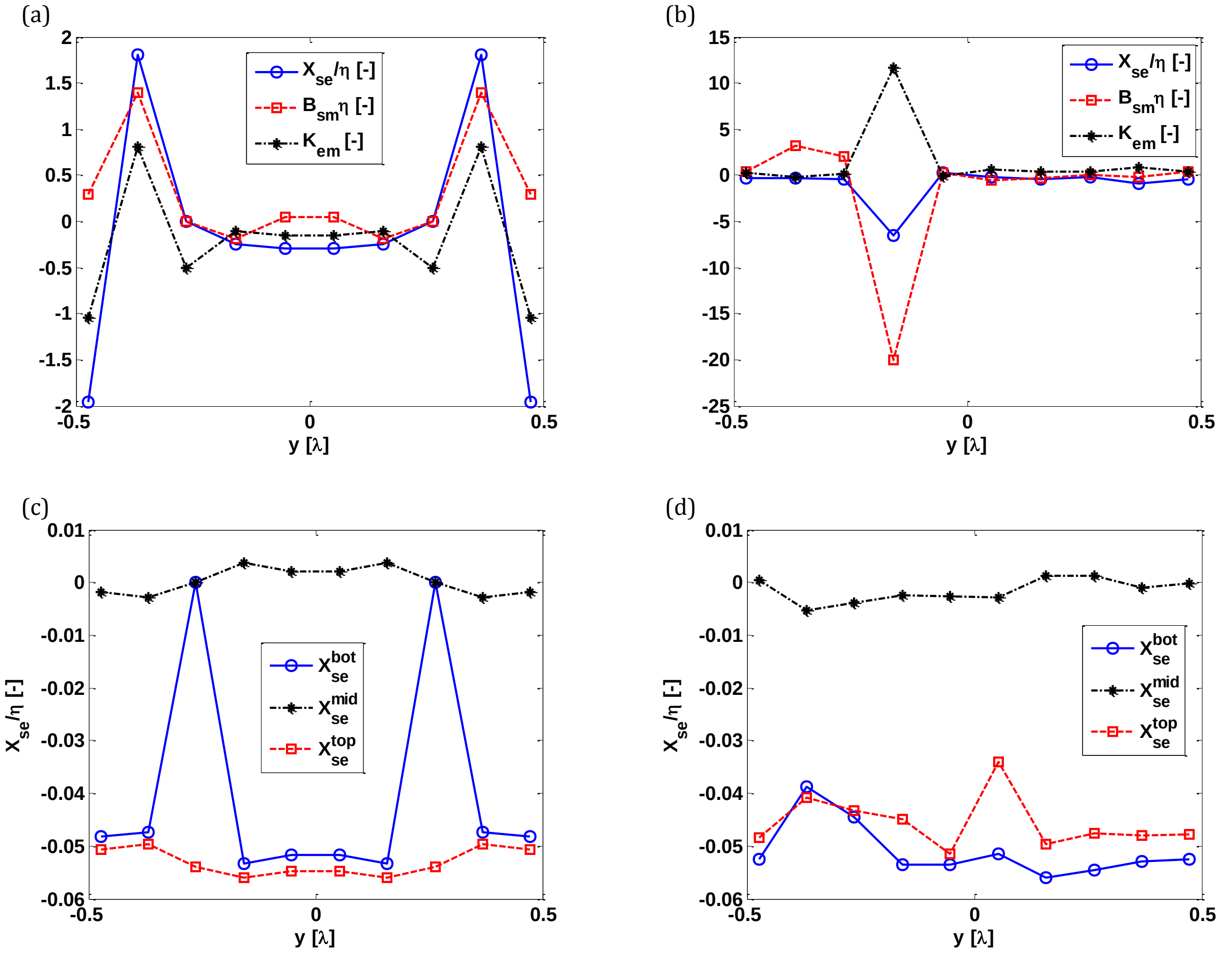


**Figure S4.** Design specifications for metasurfaces simulated in the main text (only one period is presented). Metasurface constituents for (a) beam splitting application and (b) perfect reflection application. Three-sheet reactance values as per Eq. (S5) for (c) beam splitting metasurface and (d) perfect reflection metasurface.
